# Supplementary material for: Train An Imaginative Agent
Source: arXiv:2610.26845 source file (2026-10-19)
Supplement: Supplementary file 1 [file contents.tex]

\makeatletter
\let\app@originaladdcontentsline\addcontentsline
\renewcommand{\addcontentsline}[3]{%
  \app@originaladdcontentsline{#1}{#2}{#3}%
  \begingroup
    \def\app@extension{#1}%
    \def\app@toc{toc}%
    \ifx\app@extension\app@toc
      \addtocontents{apc}{%
        \protect\contentsline{#2}{#3}{\thepage}{\@currentHref}%
      }%
    \fi
  \endgroup
}
\definecolor{appendixblue}{RGB}{35,76,132}
\section*{\textcolor{appendixblue}{Appendix Contents}}
\phantomsection
\pdfbookmark[0]{Appendix Contents}{appendix.contents}
\label{app:contents}
\par\medskip
\begingroup
  \setcounter{tocdepth}{2}
  \color{appendixblue}
  \hypersetup{colorlinks=true,linkcolor=hyperlinkblue,linktoc=all}
  \@starttoc{apc}
\endgroup
\makeatother
